# Supplementary material for: Using Limited Neural Networks to Assess Relative Mechanistic Influence on Shock Heating in Granular Solids
Source: arXiv:2305.07660 source file (2023-04-27)
Supplement: Supplementary file 1 [file Supplemental_Material.pdf]

# Supplemental Material to: Using Limited Neural Networks to Assess Relative Mechanistic Influence on Shock Heating in Granular Solids

Brenden W. Hamilton, Timothy C. Germann
Theoretical Division, Los Alamos National Laboratory, Los Alamos, New Mexico 87545, USA

**SM-1: Extended MD Methods**

Initial simulations cells, built with the PBXGen algorithm[i], consist purely of TATB grains. The cell is set to be thin in the Z direction, which is periodic. Grains are columnar along the Z axis, and all grains are crystallographically set that the [001] direction is long Z. The X-Y face is randomly oriented for each grain to increase anisotropy.

PBXGen is initialized to insert a bimodal distribution of grains with peak sizes at 40 nm and 8 nm. In both systems generated, the larger grains account for roughly 2/3 of the total mass. The two cells final structure are sizes of 100 x 400 nm (12440592 atoms) and 100 x 200 nm (6183984 atoms).

As PBXGen packed particles typically only have a volumetric packing density of around 50%, the initial cell sizes were 200x400 nm and 200x200 nm. The X direction was then compacted to the final size over a period of 250 ps. Temperature was set 500 K to promote grain boundary formation and help anneal defects formed during compaction. Atom coordinates were fractionally remapped at every step during compaction. The final cells were thermalized at 300 K for 25 ps.

Shock simulations were conducted along the Y axis (long direction) using a momentum mirror on the bottom box boundary and a free boundary at the top. The X and Z directions remained periodic.

All trajectory analysis for building training and testing sets were done on a molecular basis. The molecule center of mass was used for position, and the center of mass velocity for velocity. We define C.O.M. properties with capital letters and atomic properties with lowercase letters. From the per atom velocities, we compute three kinetic energy values: the total, translational, and roto-vibrational:

$$KE_{Tot} = \sum \frac{1}{2} m_i (v_i \cdot v_i)$$
$$KE_{Trans} = \frac{1}{2} M (V_i \cdot V_i)$$
$$KE_{ro-vib} = KE_{Tot} - KE_{Trans}$$

Where m and M are atomic and molecular mass, and v and V are velocity vectors. Subscript i designates each atom, which the sum is over. Temperature is defined as the roto-vibrational kinetic energy in units of kelvin from the classical specific heat:

$$KE_{ro-vib} = \frac{3N-3}{2} k_B T$$

The composite trajectory frame is taken as molecular properties at the time for each molecule of $t_o$ + 5 ps where $t_o$ is the time in which the molecule is shocked. We define shocked time as the first frame in which a molecule has a C.O.M. velocity between -0.3 and 0.3 km/s for three consecutive frames (0.3 ps). This ensures that the molecule is at rest, which is shocked in the reverse ballistic frame used here. Additionally, molecules that are pushed into a void are treated as shocked only after material has recompressed on the downstream face of a pore. This leads $t_o$

+ 5 ps to be a measure of 5 ps after shock heating. This minimizes the effects from local thermal transport and pressure relaxation events.

**SM-2: Extended ML Methods**

Neural networks are defined to have a variable sized input and hidden layer. The input layer is of size N+1, where N is the number of neighbor bins used. The hidden layer is over size $\lfloor 0.5(N+1) \rfloor$. For the no nearest neighbor case (N+1=1), the input and hidden layer are set to have size of 1. A sigmoid function is used from input to the hidden layer. The output layer is always size one, and a linear function connects the hidden and output layer. A biasing value is allowed for both functions.

The larger of the two MD systems is used as the training set. An 80-20 split is used during training. An early stopping criterion is set to stop training and take the best network if the mean square error of the 20% testing group does not drop by at least 0.00001 over 100 epochs. This error delta is in normalized units, where all input/output data is utilized as the Z-score of the data. An Adam optimizer[ii] is used with a $1 \times 10^{-3}$ learning rate. All errors values presented in this work are based on predictions of the smaller of the MD systems which is not included in training at all.

Within the input layer for a given network, the order of the bins is constant in the input layer, such that the network can differentiate upstream and downstream of the bin, as well as some information regarding shape of a pore.

**SM-3: Temperature Prediction Heat Maps**

Bin = 2.5 nm, 5 NN

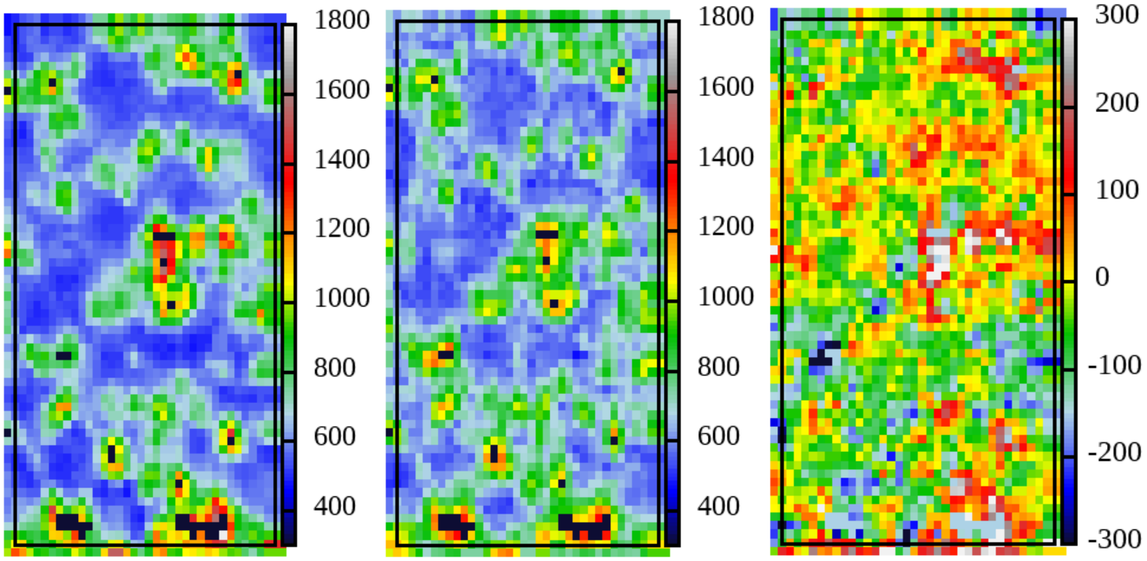

Bin = 2.5nm, 1 NN

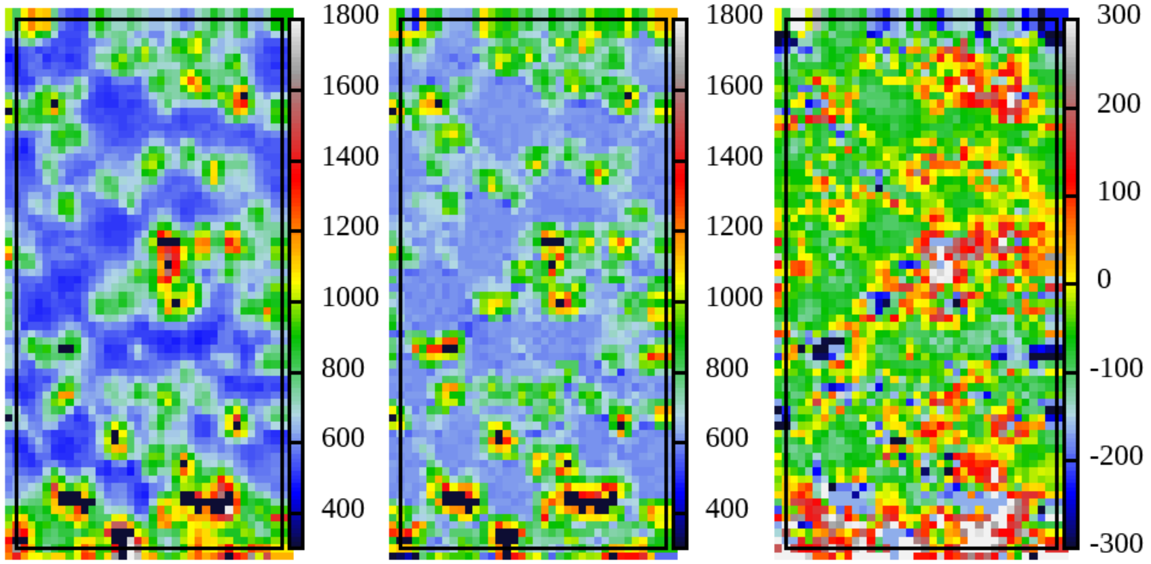


Bin = 3.0nm, 8 NN

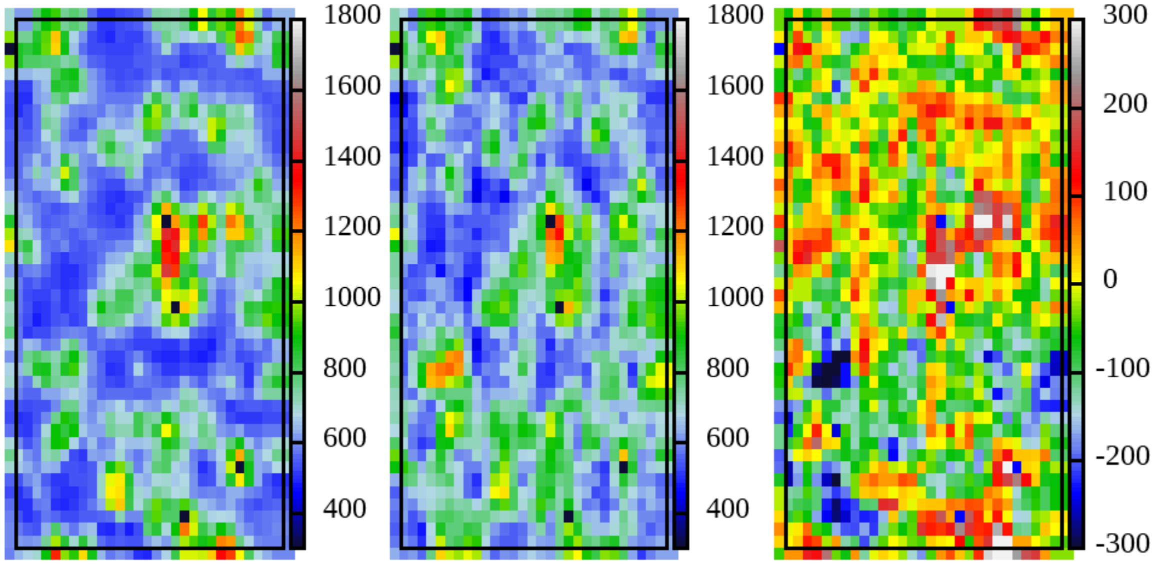

Bin=3.0nm, 4 NN

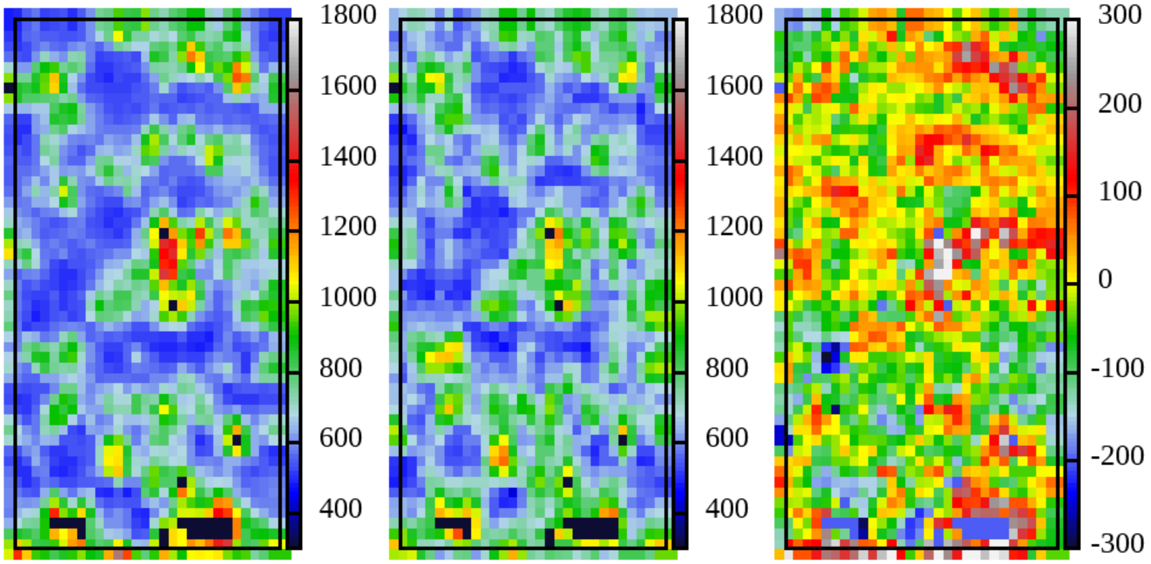


Bin = 3.0nm, 1 NN

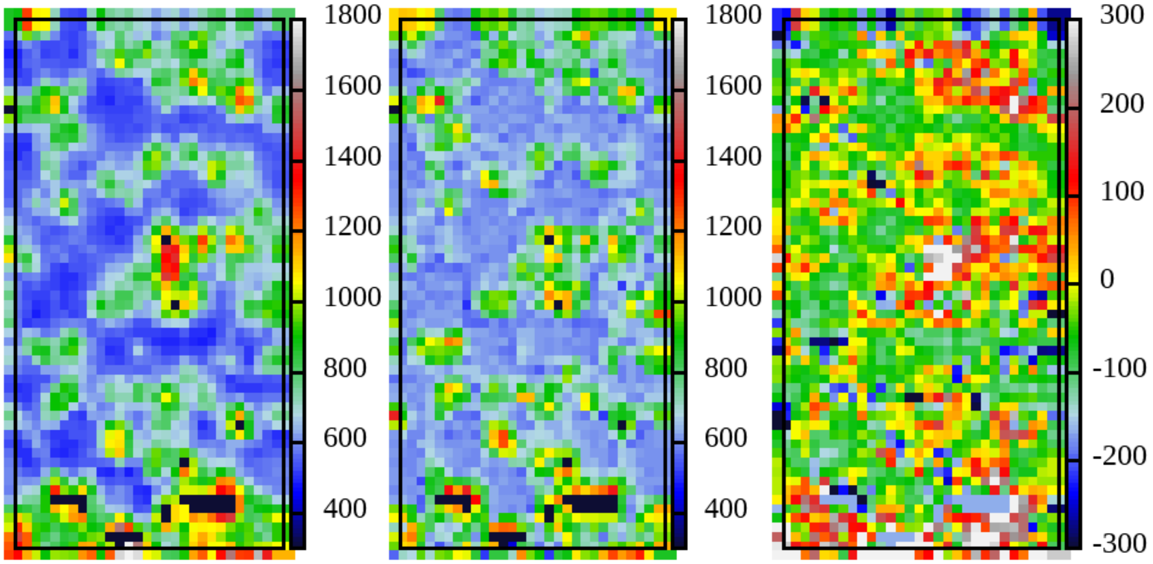

Bin = 4.0nm, 6 NN

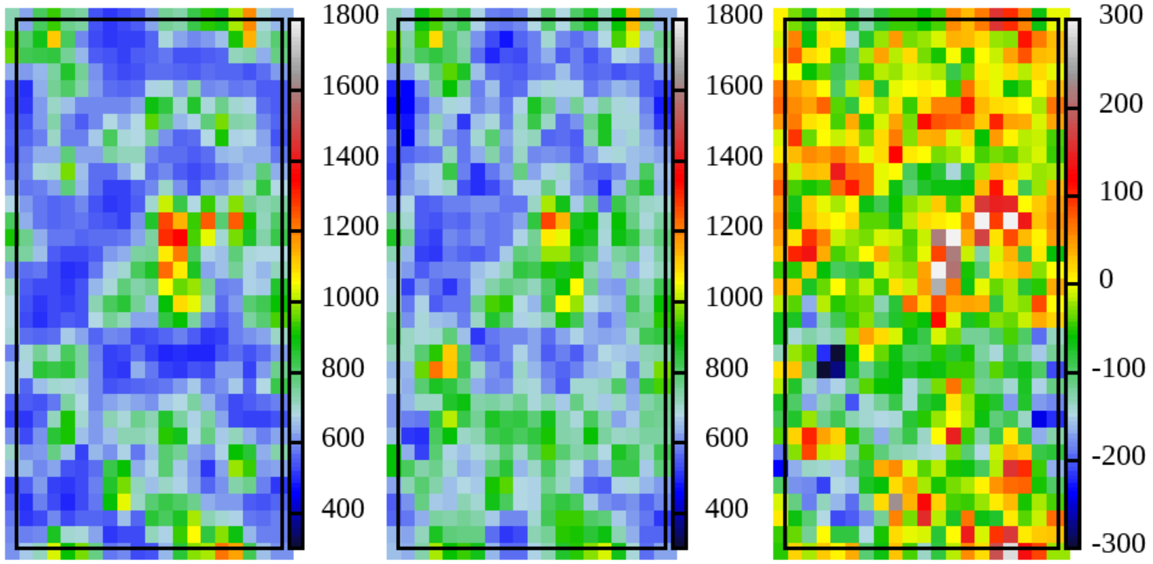


Bin = 4.0nm, 3 NN

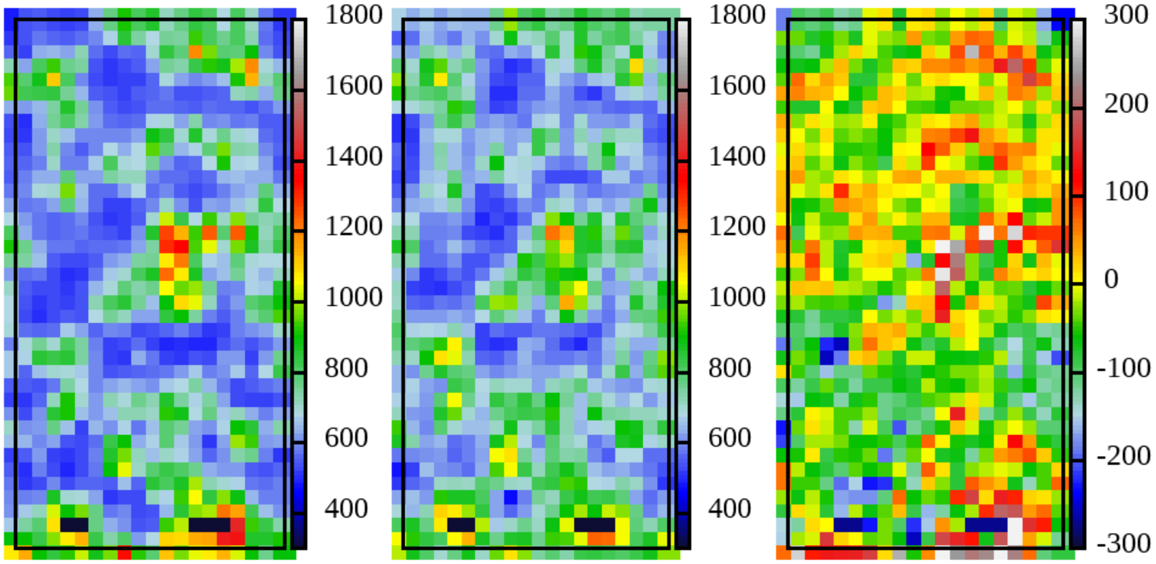

Bin = 4.0nm, 1 NN

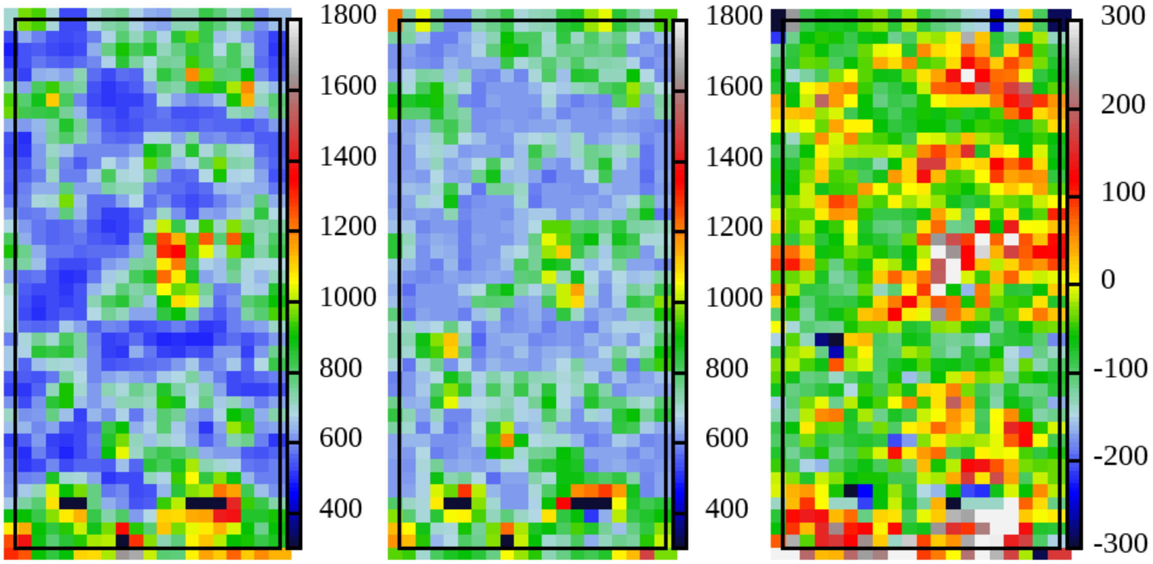


Bin = 5.0nm, 6 NN

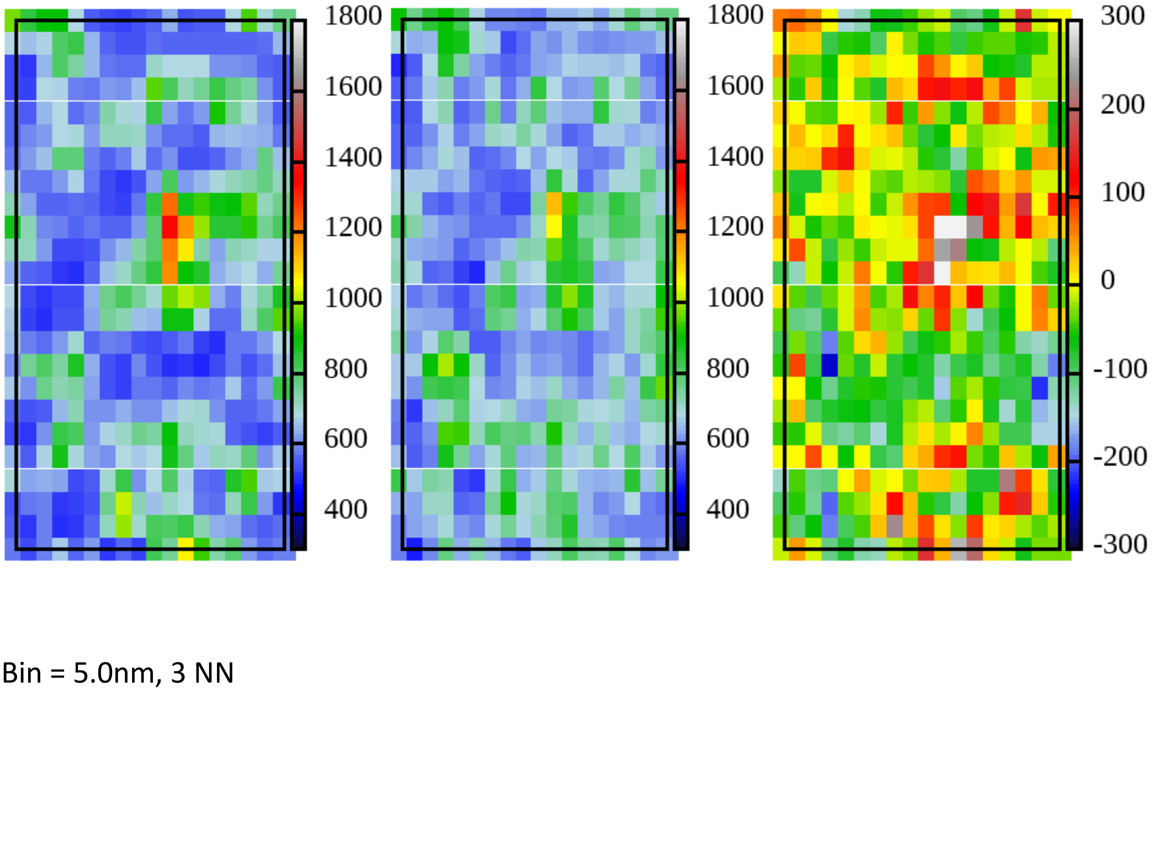


Bin = 5.0nm, 3 NN

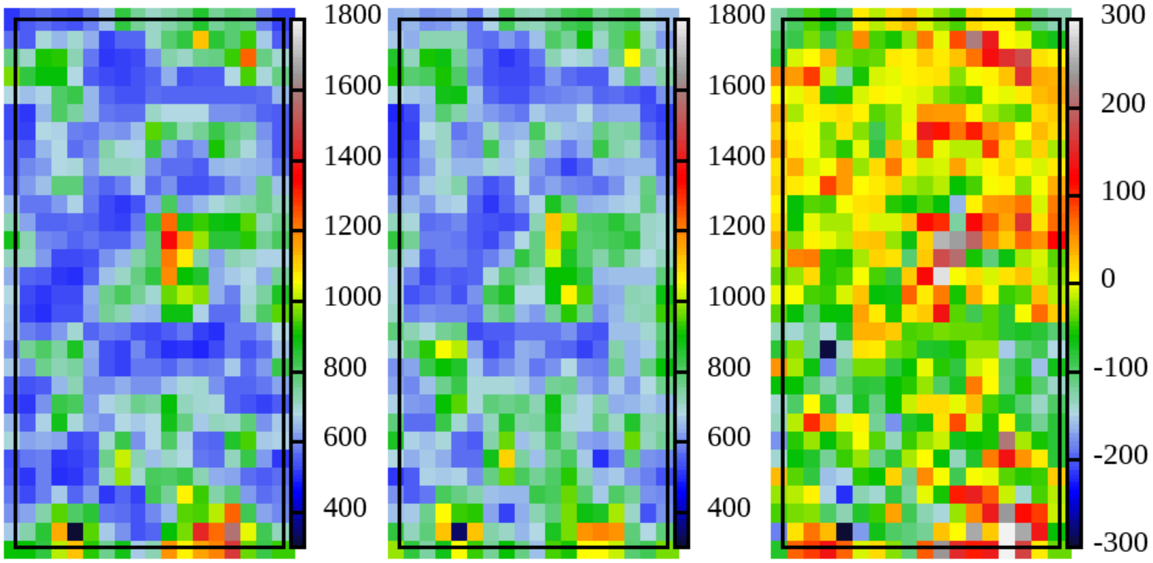
1800
1600
1400
1200
1000
800
600
400
1800
1600
1400
1200
1000
800
600
400
300
200
100
0
-100
-200
-300

Bin = 5.0nm, 1 NN

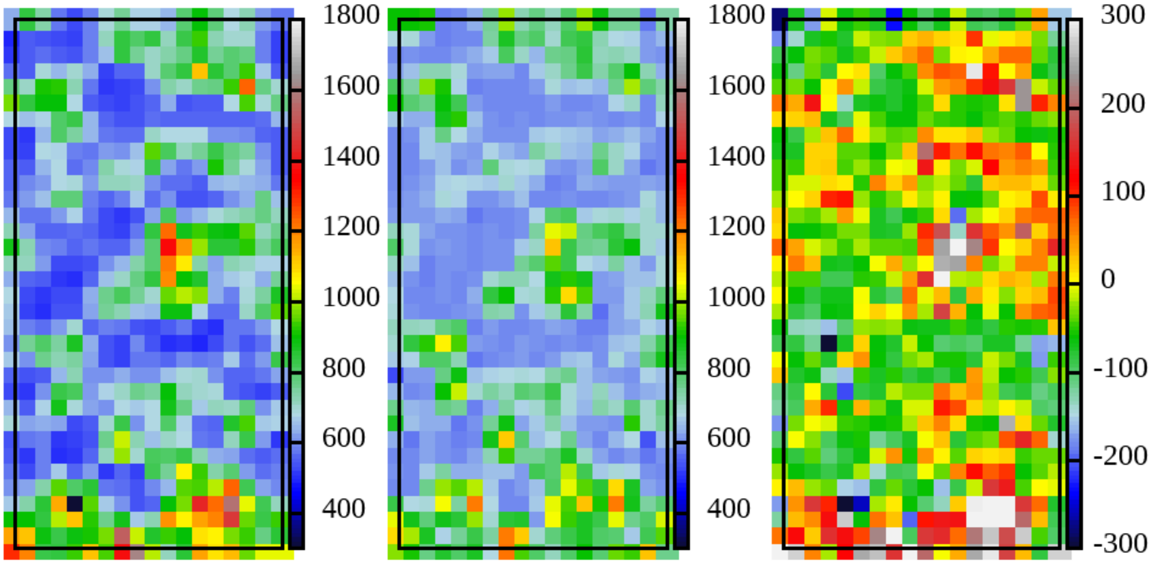
1800
1600
1400
1200
1000
800
600
400
1800
1600
1400
1200
1000
800
600
400
300
200
100
0
-100
-200
-300

**SM-4: $U_{Latent}$ Prediction Heat Maps**

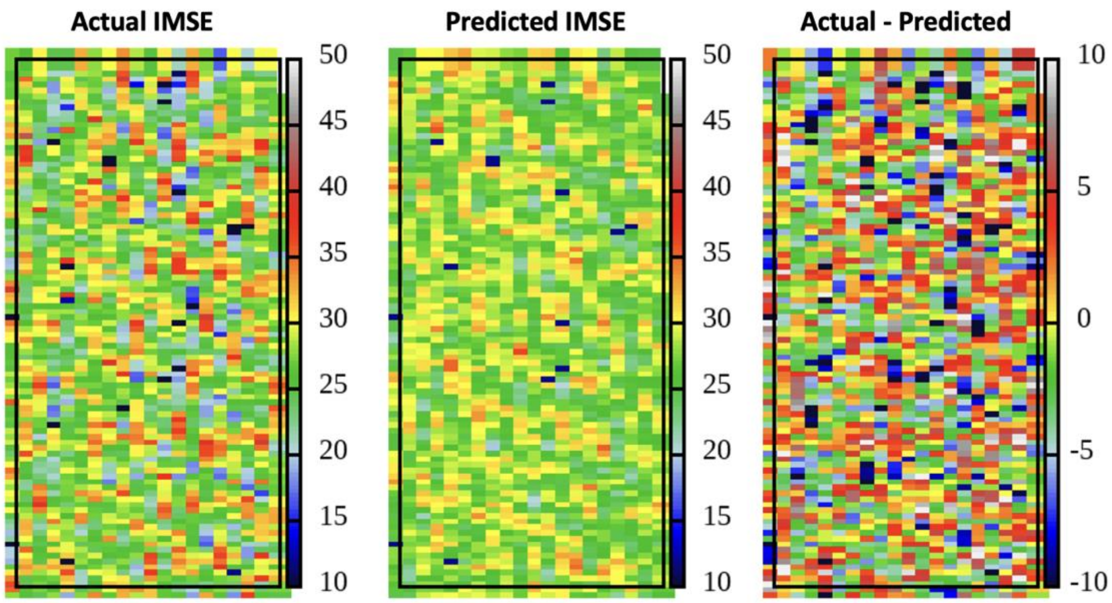


SM Figure XXX:

**SM-5: $U_{Latent}$ RMSE Values**

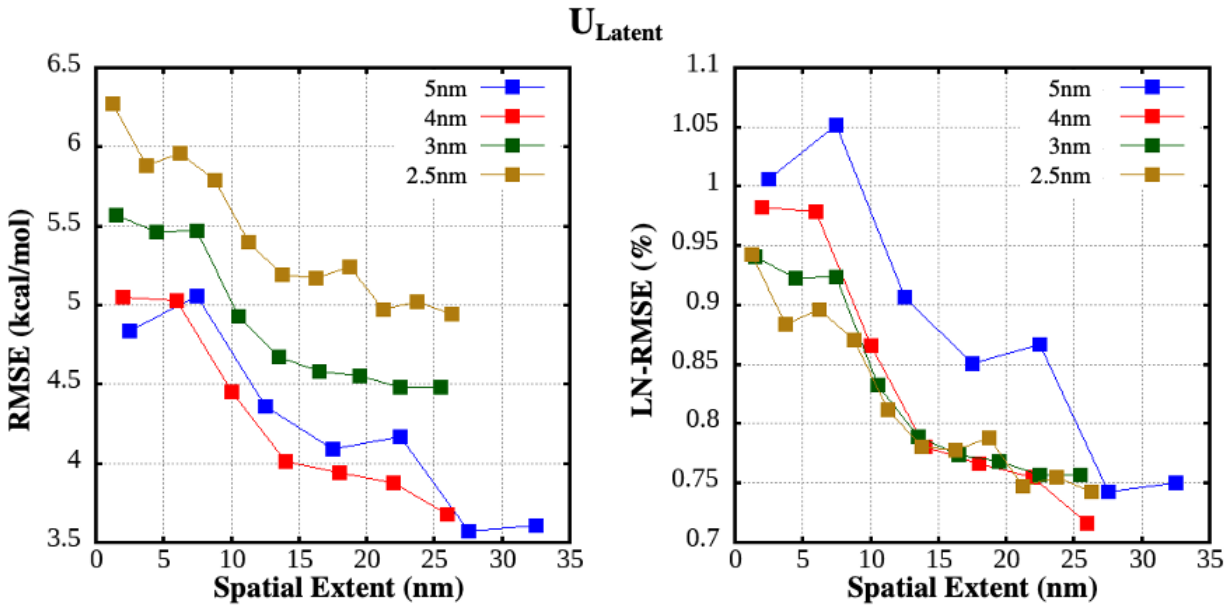


**References**

[i] Li, C., Hamilton, B. W., Shen, T., Alzate, L., & Strachan, A. (2022). Systematic Builder for All-Atom Simulations of Plastically Bonded Explosives. Propellants, Explosives, Pyrotechnics, 47(8), e202200003.
[ii] Kingma, D. P., & Ba, J. (2014). Adam: A method for stochastic optimization. arXiv preprint arXiv:1412.6980.
